# Supplementary material for: Flux Backgrounds and Exceptional Generalised Geometry
Source: arXiv:1808.04225 source file (2018-08-13)
Supplement: Supplementary file 1 [file AppGamma.tex]

\documentclass[debug]{phd}

\begin{document}
	\chapter{Gamma matrices conventions}
		\section{Introduction and preliminaries}
			\subsection{Introduction}
				\dots
		\section{G-structures}
			\subsection{G-structures}
				\ldots
			\subsection{Almost complex structures}
				\ldots
			\subsection{Presymplectic structures}
				\ldots
			\subsection{Hermitian manifolds}
				\ldots
			\subsection{Parallelisable manifolds}
				\ldots
		\section{Holonomy and Torsion}
			\ldots
			\subsection{Definitions}
				\ldots
			\subsection{Integrability of structures}
				\ldots
			\subsection{Examples: Calabi-Yau and Sasaki-Einstein manifolds}
				\ldots
				\subsubsection{Calabi-Yau manifolds}
					\ldots
				\subsubsection{Sasaki-Einstein manifolds}
					\ldots
\end{document}
